# Supplementary material for: Recurrence and transience for the frog model on trees
Source: arXiv:1404.6238 ancillary file (2016-05-17)
Supplement: Supplementary file 1 [file code_explanation.pdf]

## DOCUMENTATION FOR FROG.SAGE

CHRISTOPHER HOFFMAN, TOBIAS JOHNSON, AND MATTHEW JUNG

ABSTRACT. Our proof of Theorem 1 (ii) in *Recurrence and transience for the frog model on trees* depends on a computer calculation performed by `frog.sage`. This document provides a guide to the source code and explains the steps we took to make sure the calculation is free of errors.

Our proof of Theorem 1 (ii) involves finding the entries of a  $27 \times 27$  matrix  $\Phi(\theta)$  and then computing its eigenvalues. We carried this out with a program `frog.sage` that accompanies this document. The source code itself contains basic instructions for checking the results of the paper. Here, we provide a guide to the program on a higher level.

There are three steps to the calculation:

- (1) From each of the 27 initial states given by  $P(a, b, c)$  for  $1 \leq a \leq 3$  and  $0 \leq b, c \leq 2$ , compute all possible states to which the frog model on  $\mathbb{T}_5$  can transition in two steps, as well as the exact probabilities of doing so.
- (2) Represent every ending state as a collection of particles of our 27 types, at levels  $-2$ ,  $0$ , and  $2$  from the initial particle.
- (3) Compute the matrix  $\Phi(\theta)$  exactly. For some given value of  $\theta$ , confirm that its highest eigenvalue in absolute value is less than 1.

We have provided two implementations of Step 1, in the functions `FrogSpace.advance_fast` and `FrogSpace.advance_slow`. Using the faster one, the entire calculation takes a few seconds. Here, we took advantage of symmetries to simplify things. Starting from the  $P(3, 0, 0)$  state, for example, each frog has six choices for where to move. Considering all 216 outcomes after one step, however, is unnecessary: most are equivalent. Our approach was to consider the first frog as moving backward with probability  $1/6$ , and moving forward to child 1 with probability  $5/6$ , on the grounds that moving to any other of the five children would give an equivalent state from our perspective. When the first  $k$  children of a frog's location have been visited and the other  $5 - k$  have not, we consider the frog to move backwards with probability  $1/6$ , forward to each of the  $k$  visited children with probability  $1/6$ , and forward to the *first* of the unvisited children with probability  $(5 - k)/6$ . This algorithm could still be improved considerably. It fails to take advantage of the symmetries obtained by permuting the order of the frogs, for example.

While this algorithm is simple enough, our other one is still simpler. In `FrogSpace.advance_slow`, to compute the two-step transition probabilities from some particle, we first compute all possible outcomes after one step, allowing all frogs any of their six moves. Then, we repeat for one more step. This is spectacularly inefficient, but it is easy to see that it is coded correctly, and it serves as a useful check for our faster algorithm. Though it was too memory intensive to do the entire calculation using this algorithm, we confirmed that for  $P(a, b, c)$  with  $a \leq 2$ , it gives identical results to faster algorithm.

Step 2 is more straightforward. In our code, this is done by the function `identify_types`. For each ending state found in Step 1, we loop through all vertices containing frogs. For each one, we count how many frogs are at that vertex, how many sibling vertices have no sleeping frog, and how many child vertices have no sleeping frogs. Then we represent the ending state as a collection of particles based on this. When there are four or more frogs at a vertex, we represent the frogs by as many  $P(3, b, c)$  particles as possible, along with an additional  $P(a, b, c)$  particle with  $a \leq 2$  if necessary.

In Step 3, the exact computation of  $\Phi(\theta)$  as a symbolic expression in terms of  $\theta$  occurs in the function `get_matrix`. We substituted  $\alpha$  for  $e^{-\theta}$  to simplify the expressions. Checking that the highest eigenvalue was less than one for a given choice of  $\theta$  offered up a few computational issues. In our paper, we describe how we substituted  $\theta = \log 3$  to get a matrix of rationals, which successively squared until all of its row sums were bounded by 1. In our code, we have provided a function `infinity_norm` that computes the maximum absolute row sum of a matrix. We have also given a function `highest_eigenvalue` which just computes eigenvalues numerically using the library `numpy`.
